# Supplementary material for: Compositional Generalization Requires Compositional Parsers
Source: arXiv:2202.11937 source file (2022-02-24)
Supplement: Supplementary file 1 [file few_gen_type_eval_appendix.tex]

\begin{table*}
      \centering 
      \tiny % \tiny \scriptsize \footnotesize \small \normalsize
      \setlength{\tabcolsep}{2pt}
      
          \begin{tabular}{@{}llccc|cccccc|c|c@{}}
          	\toprule
          	                                      &                               &                                                 \multicolumn{9}{c|}{semantic}                                                 & \multicolumn{2}{c}{syntactic} \\
          	\cmidrule(lr){3-11} \cmidrule(l){12-13} &                               &   \amBert   & \amBert+\dist &    LeAR     & Lex:Simple  &   mT5 xl    &   conklin   &   csordas    &    BART    &  BART+syn   &   Benepar   &      BART       \\
          	Class                                 & Generalization type           &  train100   &   train100    &    train    &    train    &    train    &  train100   &   train100   &  train100  &  train100   &  train100   &    train100     \\ \midrule
          	\structg                              & objPP to subjPP               & \asbar{49}  &  \asbar{78}   & \asbar{93}  &  \asbar{0}  &  \asbar{0}  &  \asbar{0}  & \asbar{0} & \asbar{0}  &  \asbar{0}  & \asbar{84}  &    \asbar{1}    \\
          	                                      & CP recursion                  & \asbar{100} &  \asbar{100}  & \asbar{100} &  \asbar{0}  &  \asbar{0}  &  \asbar{0}  &  \asbar{0}   & \asbar{0}  &  \asbar{7}  & \asbar{95}  &    \asbar{4}    \\
          	                                      & PP recursion                  & \asbar{41}  &  \asbar{99}   & \asbar{99}  &  \asbar{1}  & \asbar{10}  &  \asbar{0}  &  \asbar{0}   & \asbar{10} &  \asbar{8}  & \asbar{98}  &    \asbar{8}    \\ \midrule
          	\propg                                & prim. to obj. (proper)  & \asbar{85}  &  \asbar{94}   & \asbar{93}  & \asbar{66}  & \asbar{84}  &  \asbar{0}  &  \asbar{64}  & \asbar{55} & \asbar{98}  & \asbar{99}  &   \asbar{97}    \\
          	                                      & subj. to obj. (proper)    & \asbar{90}  &  \asbar{96}   & \asbar{93}  & \asbar{64}  & \asbar{86}  &  \asbar{67} &  \asbar{60}  & \asbar{86} & \asbar{95}  & \asbar{100} &   \asbar{94}    \\
          	\lexg                                 & All 16 other types            & \asbar{100} &  \asbar{100}  & \asbar{100} & \asbar{100} & \asbar{100} &  \asbar{94} &  \asbar{90}  & \asbar{99} & \asbar{100} & \asbar{100} &   \asbar{96}    \\ \midrule[\heavyrulewidth]
          	                                      & Overall                       & \asbar{94}  &  \asbar{98}   & \asbar{99}  & \asbar{82}  & \asbar{85}  &  \asbar{75} &  \asbar{76}  & \asbar{83} & \asbar{86}  & \asbar{99}  &   \asbar{83}    \\ \bottomrule
          	                                      &                               &             &               &
          \end{tabular}

    \caption{Exact match accuracies on the individual generalization types. We have compressed all 16 generalization types of the \lexg class into a single row and report the average accuracy.
    Additionally to our own runs we copy numbers from \citet[Lex:Simple]{akyurek-andreas-2021-lexicon},  \citet[mT5 xl]{orhan-2021-compgen} and run own train100 experiments \yy{(1 run)} for \citet[\yy{model  config?}]{conklin-etal-2021-meta} and \citet[\yy{model  config?}]{csordas-etal-2021-devil}. 
    \pw{we might have two tables like this: one with all possible details in the appendix, and a condensed version in the main paper.}
    }\label{tab:appendix_selected_gentype_eval}
  \end{table*}

%%% Local Variables:
%%% mode: latex
%%% TeX-master: "../main"
%%% End:
